# Supplementary material for: Capacity of All Nine Models of Channel Output Feedback for the Two-user Interference Channel
Source: arXiv:1104.4805 source file (2013-01-25)
Supplement: Supplementary file 1 [file apa.tex]

\subsection{Outer bounds in terms of $\mathsf{SNR}$ and $\mathsf{INR}$}
\label{apa}
In order to represent the bounds (\ref{eq:finalg}) and
(\ref{eq:finalg2}) in terms of $\mathsf{SNR}$ and $\mathsf{INR}$, the
variance of conditioned random variable is bounded using Schur's
complement \cite{schur} and its corresponding entropy is bounded by
the entropy of the Gaussian random variable for the computed
variance \cite{coverbook}. Assume that the correlation between $X_1$
and $X_2$ is $\rho$, i.e. $\rho =
\mathsf{E}[X_1{X_2}^*]$.  The variance of the received symbol $Y_1$ is
upper bounded by $\mathrm{var}[Y_2] \leq \mathsf{E}[|Y_1|^2] = |g_d|^2
+ |g_c|^2 + 2\mathrm{Re}(\rho g_d{g_c}^*) + 1$. Therefore
\begin{equation}\label{eq:apa1}
\frac{1}{N}\sum_{i = 1}^N h(Y_{1i}) \leq \log2\pi e(1 + \mathsf{SNR +
INR} + 2|\rho|\sqrt{\mathsf{SNR. INR}} ).
\end{equation}
Also,
\begin{equation}
\mathsf{E}[|S_2|^2] = |g_c|^2\mathsf{E}[|X_2|^2] + \mathsf{E}[|Z_1|^2]  =
|g_c|^2 + 1 = \mathsf{INR} + 1.
\end{equation}

The variance of a $Y_{2}$ conditioned on $S_2$ is bounded by
\begin{eqnarray*}
&\mathrm{var}[Y_2| S_2] & \leq \mathsf{E}[|Y_2|^2] -
\frac{\mathsf{E}[Y_2S_2^*].\mathsf{E}[Y_2^*S_2]}{\mathsf{E}[|S_2|^2]}\\
 & = & 1 + |g_d|^2 + |g_c|^2 + 2\mathrm{Re}(\rho^* g_dg_c^*) -
\frac{|g_cg_d|^2 + |g_c|^4\rho^2 + 2|g_c|^2 \mathrm{Re}(g_c^*g_d
\rho^* )}{|g_c|^2 + 1} \\
& =& 1 + \frac{|g_c|^4 (1 -\rho^2) + |g_c|^2 + |g_d|^2 + 2\mathrm{Re}(g_c^*g_d\rho^*)}{|g_c|^2 + 1}
\end{eqnarray*}
and  substituting for $|g_d|^2 = \mathsf{SNR}, |g_c|^2 =
\mathsf{INR}, \mathrm{Re}(\rho^*g_c^*g_d)=
|\rho|\sqrt{\mathsf{SNR.INR}}$, the corresponding entropy is
\begin{equation}\label{eq:apa2}
\frac{1}{N} \sum_{i = 1}^N h(Y_{2i}| S_{2i}) = \log2\pi e\left(1 + \mathsf{INR} + \frac{\mathsf{SNR} - (1 + |\rho|^2) \mathsf{INR} + 2 |\rho| \sqrt{\mathsf{SNR.INR} }}{1+ \mathsf{INR}}\right)
\end{equation}
Using Schur's complement, $\mathrm{var}[Y_1|X_2 S_1]$ is bounded
as
\begin{eqnarray*}
\mathrm{var}(Y_1|X_2 S_1) \leq \mathsf{E}[|Y_1|^2] - K_{Y_1(X_2, S_1)} K_{(X_2, S_1)(X_2,S_1)}^{-1} K^*_{Y_1(X_2 S_1)}
\end{eqnarray*}
where $\mathsf{E}[|Y_1|^2]  = 1 + |g_d|^2 + |g_d|^2 + 2\mathrm{Re}(\rho^*g_c^*g_d)$ and
\begin{displaymath}
 K_{(X_2, S_1)} = \left[    \begin{array}{cc}
 1 & g_c^*\rho^* \\
 g_c\rho & |g_c|^2 + 1 \end{array} \right]
\end{displaymath} and
\begin{displaymath}
K_{Y_1(X_2,S_1)}  = \left[  \begin{array}{cc} g_d^*\rho^* +g_c* & g_cg_d^* + |g_c|^2\rho \end{array}\right].
\end{displaymath}
Then,
\begin{equation}\label{eq:apa3}
\frac{1}{N}\sum_{i =1}^N h(Y_{1i}| X_{2i} S_{1i}) \leq \log2 \pi e\left( 1 + \frac{(1 - |\rho|^2)\mathsf{SNR}}{1 + (1 - |\rho|^2) \mathsf{INR}} \right)
\end{equation}
Since the noise is distributed as $\mathcal{CN}(0,1)$, 
\begin{equation}\label{eq:apa4}
h(Z_1) = h(Z_2) = h(Z_3) = \log(2 \pi e).
\end{equation}
Combining \eqref{eq:apa1}, \eqref{eq:apa3} and
\eqref{eq:apa4}, the following outer-bounds are obtained
\begin{equation}
R_1 + R_2 \leq \sup_{0 \leq |\rho| \leq 1} \left\{ \log \left( 1 +
\frac{(1 - |\rho|^2) \mathsf{SNR}}{1 + (1 - |\rho|^2)
\mathsf{INR}}\right) + \log (1 + \mathsf{SNR + INR} +
2|\rho|\sqrt{\mathsf{SNR. INR}} )\right\}.
\end{equation}
\begin{eqnarray}
2R_1 + R_2 & \leq & \sup_{0 \leq |\rho| \leq 1} \{ \log \left( 1 +
\frac{(1 - |\rho|^2) \mathsf{SNR}}{1 + (1 - |\rho|^2)
\mathsf{INR}}\right) + \log (1 + \mathsf{SNR + INR} +
2|\rho|\sqrt{\mathsf{SNR. INR}} ) + \nonumber \\
&& \log\left(1 + \mathsf{INR} + \frac{\mathsf{SNR} - (1 +
|\rho|^2) \mathsf{INR} + 2 |\rho| \sqrt{\mathsf{SNR.INR} }}{1+
\mathsf{INR}}\right) \}
\end{eqnarray}
