# Supplementary material for: Capacity of All Nine Models of Channel Output Feedback for the Two-user Interference Channel
Source: arXiv:1104.4805 source file (2013-01-25)
Supplement: Supplementary file 2 [file apd_a.tex]

\subsection{Achievable strategy for the corner points of the capacity region}
\label{apd_a}

\begin{center}
\textbf{Strong interference regime}
\end{center}
We will now show the achievability for the two corner points in the
case of strong interference ($m > n$).

\paragraph{Corner point intersecting the bounds of
\underline{${R_2}$ and ${R_1 + R_2}$}} In this case, the desired
corner point is $(0,m)$. Note that since $\mathsf{T_1}$ is not sending
any message of its own, we can convert this to an effective relay
channel, where there is a direct link between $\mathsf{T_2}$ and
$\mathsf{D_2}$ while there is a relay that receives $Y_1$ and sends
$X_1$. Thus, the decode and forward strategy \cite{relay} for the
relay channel can be used to achieve this corner point.

\paragraph{Corner point intersecting the bounds of
\underline{${R_1}$ and ${R_1 + R_2}$}} In this case, the desired
corner point is $(n, m -n)$.  For $n < m \le 2n$, this point is in the
capacity region without feedback \cite{bresler2} and thus can be
achieved with feedback. Thus, we only need to show for $m>2n$ in which
case the encoding strategy and the decoding strategy at both the
receivers is given below.

\noindent \textbf{Encoding:} In the first block, the $\mathsf{T_1}$
remains silent, while $\mathsf{T_2}$ generates i.i.d. $X_{21,p}$ and
$X_{21,r}$ such that $|X_{21,p}| = n, |X_{21,r}| = m -2n $ transmits
$[X_{21,p},X_{21,r},\underbrace{0 \ldots 0}_n]^T$. From the second
block onwards, $\mathsf{T_1}$ generates i.i.d. $X_{1i,p}$ such
$|X_{1i,p}| = n$, and transmits $[X_{1i,p}, X_{2i-1,r}, \underbrace{0
\ldots 0}_n]^T$. $\mathsf{T_2}$ continues to generate and
transmit $[X_{2i,p},X_{2i,r},\underbrace{0 \ldots 0}_n]^T$.

\noindent \textbf{Decoding:} At both receivers forward decoding is
applied. Except the first block, $Y_{1i} = [X_{2i,p}, X_{2i,r},
X_{1i,p}]$ and decoding $X_{1i,p}$ is trivial. $Y_{2i} = [X_{1i,p},
X_{2i-1,r}, X_{2i,p}]^T$. Thus in each block $X_{2i-1,r}$ (relay
message of the previous block) and $X_{2i,p}$ can be decoded.

\noindent \textbf{Achievable rate:} The rate $R_1 = \frac{1}{B}\sum_{i
  = 1}(B -1)n$, and $R_2 = \frac{1}{B}\sum_{i =1}^B (Bn + (B-1)(m-
2n)) $. Letting $B \to \infty$ we get the desired rate tuple.
