# Supplementary material for: Capacity of All Nine Models of Channel Output Feedback for the Two-user Interference Channel
Source: arXiv:1104.4805 source file (2013-01-25)
Supplement: Supplementary file 3 [file apga.tex]

\subsection{Achievable rate pairs for Gaussian channel}
\label{apga}
For the $(1000)$ feedback model, we describe the power and rate
allocation to achieve rate-pairs within constant number of bits of the
corner points of the outer bound derived in Section~\ref{SecGC}. When
$\alpha \in [0,1]$, there are three non-trivial corner points in the
outer bounds, while when $\alpha \in (1, \infty)$, there exist only
two non-trivial corner points. For all non-trivial corner points in
the outer-bound, following is the rate and power allocation:

\subsubsection{Corner point: Intersection of \underline{$R_2$ and $R_1 + R_2$} bounds}\text{} \\
\paragraph{$\alpha \in [0,1]$} Following is a power split
\begin{equation} \label{ps:r2-r1r2}
\lambda_{1p} = \lambda_{2p} =
\min\left(1,\frac{1}{\mathsf{INR}}\right), \lambda_{2r} = 1 -
\lambda_{2p} \text{ and }\lambda_{1c} = \lambda_{2c} = 0.
\end{equation}
It is easy to note that the above constraints imply that there are no
common messages required to achieve any of the corner points. The
following rate allocation describes the corner point
\begin{equation} \label{rate:r2-r1r2}
R_{1p}  =  R_{2p} = \log\left(1 +
\frac{\mathsf{SNR}}{\mathsf{2INR}}\right); \text{ } R_{1r}  = R_{2r} = \log(\mathsf{INR}) - \log(3); \text{ } R_{1c}  =  R_{2c} = 0.
\end{equation}
The non existence of the common message reduces the problem of
decoding from a 3-user MAC to a 2-user MAC.

\subsubsection{Corner point: Intersection of \underline{$2R_1 + R_2$ and $R_1 + R_2$} bounds}\text{ }\\
\paragraph{$\alpha \in \left[0, \frac{1}{2}\right)$} In this regime,
the power split is identical to the power split described in
\eqref{ps:r2-r1r2}. The achievable rates too are the same as
(\ref{rate:r2-r1r2}).

\paragraph{$\alpha \in \left[\frac{1}{2}, \frac{2}{3} \right)$} In this regime we use a different power sharing strategy. Note that this choice may not
be the best in terms of providing the least gap. Nevertheless, the
corner point can be achieved within a constant number of bits for all
values of $\mathsf{SNR}$. Following is the split
\begin{equation} \label{ps:2r1r2-r1r2_2}
\lambda_{1p} = \lambda_{2p} = \min\left(1,
\frac{1}{\mathsf{INR}}\right) \text{ and } \lambda_{1c} = \lambda_{2c}
= \lambda_{1r} = \lambda_{2r} = \frac{1 - \lambda_{up}}{2}.
\end{equation}
The common and relay part share equal power, even though they do not
have the same rate. Inspired from the degrees of freedom observed from
the deterministic channel model, the following rates are chosen
\begin{eqnarray} \label{rate:2r1r2-r1r2_2}
 R_{1p} = R_{2p}  =  \log\left(1 + \frac{\mathsf{SNR}}{2\mathsf{INR}} \right); \text{ } R_{1c} = R_{2p}  =  \left\{\log\left(1 +
 \frac{\mathsf{INR}^2}{\mathsf{SNR}}\right) - \log(4)\right\}^+ \nonumber \\
 R_{1r} = R_{2r}  =  \left\{ \log\left(1 +
 \frac{\mathsf{SNR}^2}{\mathsf{INR}^3}\right) - \log\left(4\right)
 \right\}^+.
\end{eqnarray}

\paragraph{$\alpha \in \left[\frac{2}{3}, 1\right]$} From the intuitions
developed in the deterministic channel, corner point in this regime
will be shown to be achievable \emph{without} feedback. We do not use
any relay messages here and do not follow the achievability strategy
proposed in Section \ref{subsec:onelink_a_l}. We use private and
common messages and use following power sharing
\begin{equation} \label{ps:2r1r2-r1r2_3}
\lambda_{1p} = \lambda_{2p} = \min\left(1,\frac{1}{\mathsf{INR}}\right) \text{ and }
\lambda_{1c} = \lambda_{2c} =  1 - \lambda_{1p} \text{ and }
\lambda_{1r} = \lambda_{2r}  =0.
\end{equation}
The achievable rates are as follows
\begin{equation}\label{rate:2r1r2-r1r2_3}
R_{1p} = R_{2p}  =  \log\left(1 + \frac{\mathsf{SNR}}{2 \mathsf{INR}}\right); \text{ } R_{1c}  =  \log\left(\frac{\mathsf{INR}^2}{\mathsf{SNR}} \right) -\log(3);
\text{ }  R_{2c}  = \log\left(\frac{\mathsf{SNR}}{\mathsf{INR}}\right) - \log(1.5).
\end{equation}
Notice that the decoding (if the private parts of the messages are
treated as noise) is 2-user MAC with the common parts of both the
messages to be decoded at each of the receivers following which the
private message of the intended source is decoded. %% We defer the proof
%% of the decoding feasibility of the achievable rate-tuple for this
%% corner point to Appendix \ref{cpt2}.

\subsubsection{Corner point: Intersection of \underline{$2R_1 + R_2$ and $R_1$} bounds}\text{  }\\
Again, this corner point is achievable \emph{without} feedback for all
values of $\alpha \in [0,1]$ and therefore the achievability scheme
described in \ref{subsec:onelink_a_l} is not neccessary.

\paragraph{$\alpha \in \left[0 ,\frac{1}{2}\right)$} Both $\mathsf{T}_1$ and $\mathsf{T_2}$ transmit only private messages at different rates. The power allocation is
\begin{equation}
\lambda_{1p} = 1 \text{ and } \lambda_{2p} = \min\left(1,
\frac{1}{\mathsf{INR}} \right).
\end{equation}
The remaining power at $\mathsf{T_2}$ goes unused. The corresponding
rate allocation is
\begin{eqnarray}\label{rate:2r1r2-r1_1}
R_{1p} = \log(\mathsf{SNR}) - 1 \text{ and } R_{2p} =
\log\left(\frac{\mathsf{SNR}}{\mathsf{INR}^2}\right) -1.
\end{eqnarray}
At each of the receivers the intended message is decoded by treating
the private message of the other user as noise. Thus there are two
constraints on the individual rates $R_{1p}$ and $R_{2p}.$

\paragraph{$\alpha \in \left[\frac{1}{2},1\right]$} The corner point in this
regime is within constant number of bits of the trivially achievable
rate tuple $(\log(1 + \mathsf{SNR},0)$.

\subsubsection{Corner point: Intersection of \underline{$R_1$ and $R_1 + R_2$ } bounds}
\text{} \\
\paragraph{$\alpha \in (1,2]$} The corner point is achievable without any
feedback and the power and rate allocation has been described for
completeness. The power allocation is
\begin{eqnarray}
\lambda_{1p} = \lambda_{2p} = \lambda_{1r} = \lambda_{2r} = 0; \text{ }\lambda_{1c} = \frac{\mathsf{INR}}{\mathsf{SNR}^2}, \lambda_{2c} = 1
\end{eqnarray}
and the rate allocation
\begin{equation}
R_{1p} = R_{2p} = R_{1r} = R_{2r} = 0; \text{ } R_{1c} = \log \left(1 + \frac{\mathsf{INR}}{\mathsf{SNR}}\right); \text{ }
R_{2c} = \log(\mathsf{SNR}).\label{rate:r1-r1r2_h1}
\end{equation} 

\paragraph{$\alpha \in (2, \infty)$} The power allocation strategy is
\begin{eqnarray}
\lambda_{1r} = \lambda_{2r} = \lambda_{1c} = \lambda_{2c} =
\frac{1}{2}; \text{ }\lambda_{1p} = \lambda_{2p} = 0
\end{eqnarray}
and the rate allocation 
\begin{eqnarray}
R_{1r} = R_{2r} = \log\left(\frac{\mathsf{INR}}{\mathsf{SNR}^2}\right); \text{ } R_{1c} = R_{2c} = \log(\mathsf{SNR}); \text{ }
R_{1p} = R_{2p} = 0. \label{rate:r1-r1r2_h2}
\end{eqnarray}

\subsubsection{Corner point: Intersection of $R_2$ and $R_1 + R_2$}\text{}
\\
\paragraph{$\alpha \in (1,\infty)$} The power allocation is
\begin{equation}
\lambda_{1p} = \lambda_{2p} = \lambda_{1c} = \lambda_{2c} = 0;
\lambda_{1r} = \lambda_{2r} = 1
\end{equation}
and the rate allocation is
\begin{eqnarray}\label{rate:r2-r1r2_h}
R_{1p} = R_{2p} = R_{1c} = R_{2c} = 0; \text{ }R_{1r} = R_{2r} = \log(1 + \mathsf{INR}).
\end{eqnarray}

Feasibility of the achievable rate pair is simple to show and have
been omitted for the purpose of brevity.
