# Supplementary material for: Capacity of All Nine Models of Channel Output Feedback for the Two-user Interference Channel
Source: arXiv:1104.4805 source file (2013-01-25)
Supplement: Supplementary file 4 [file aplambda_choice-shrunk.tex]

\subsection{Appropriate choice of $\mathbf{\lambda}$}
\label{apgal}
In the regime of interference, where $\alpha \in [0,1]$, 4 outer
bounds characterize the capacity region and thus there are 3 distinct
corner points. The feasibility of achievable rate tuples and power
sharing is described in Section \ref{subsec:onelink_a_l} which are
within constant gap from these corner points is shown in the first
three bullet points of this section, i.e. (\ref{cpt1}), (\ref{cpt2})
and (\ref{cpt3}). For values of $\alpha \in (1, \infty)$, 3 outer
bounds are sufficient to characterize the capacity region and thus
only two corner points are formed by the intersection of the these
bounds. The feasibility of the choice of rate tuples and power sharing
described in Section \ref{subsec:onelink_a_l} is shown in the
(\ref{cpt4}) and (\ref{cpt5}) bullets.

\subsubsection{Corner point formed by the intersection of \underline{$R_2$ with $R_1 + R_2$}, $\alpha \leq 1$}
\label{cpt1}\text{} \\

As $\lambda_{1c} = \lambda_{2c} =0$ and therefore the only decoding
constraints are on the rate $R_{1r} = R_{2r}$ (\ref{eq:dec1})
\begin{eqnarray*}
& R_{1r} \leq \log \left(1 + \frac{\lambda_r\mathsf{SNR}}{\lambda_p\mathsf{(SNR + INR) + 1} }\right) \\
\equiv & \log(\mathsf{SNR}^\alpha) - \log(3) \leq \log\left(\mathsf{SNR}^\alpha\frac{\mathsf{SNR} + 2}{\mathsf{SNR} + 2\mathsf{SNR}^\alpha}  \right) \\
\equiv & 0 \leq 2(\mathsf{SNR -  SNR^\alpha}) + 6
\end{eqnarray*}
It is easy to show that the above holds for $\alpha \in [0, 1)$. The
other constraint on $R_{1r}$ (\ref{eq:2mac})
\begin{eqnarray*}
& R_{1r} \leq \log\left( 1 +
\frac{\lambda_r\mathsf{SNR}^\alpha}{\lambda_p \mathsf{INR + 1}} \right) \\
\equiv & \log(\frac{\mathsf{SNR^\alpha}}{3}) \leq \log\left( \frac{1 + \mathsf{SNR}^\alpha}{2}\right).
\end{eqnarray*}
The constraint on $R_{1p} = R_{2p}$ is
\begin{eqnarray*}
& R_{1p} = R_{2p} \leq \log\left(1 + \frac{\lambda_p \mathsf{SNR}}{\lambda_p \mathsf{INR} + 1}\right) \\
\equiv & \log\left(1 + \frac{\mathsf{SNR}}{\mathsf{2INR}} \right) \leq \log\left(1 + \frac{\mathsf{SNR}}{\mathsf{2INR}} \right)
\end{eqnarray*}

\subsubsection{Corner point formed by the intersection of \underline{$R_1+R_2$ with $2R_1 + R_2$}, $\alpha \leq 1$}\label{cpt2}

\paragraph{$\alpha \in \left[0, \frac{1}{2}\right)$} Since the choice of achievable rate tuple is same as \eqref{rate:r2-r1r2}, its feasibility is already proven.

\paragraph{$\alpha \in \left[\frac{1}{2}, \frac{2}{3}\right)$} In this regime, the achievable corner point \eqref{rate:2r1r2-r1r2_2} has $R_{1r} = \left\{ \log\left(1 +
\mathsf{SNR}^{2-3\alpha}\right) - \log(4) \right\}^+ $. We show that $\left\{ \log\left(1 +\mathsf{SNR}^{2-3\alpha}\right) - \log(3)\right\}^+$ satisfies constraint
\begin{eqnarray*}
& R_{1r} \leq \log \left( 1 +
\frac{\lambda_{r}\mathsf{SNR}}{\lambda_p\mathsf{(SNR + INR) + 1}}
\right) \\
 \equiv & \log\left(1 + \mathsf{SNR}^{2-3\alpha}\right) -
\log\left(3\right) \leq \left( 1 +
\frac{\mathsf{SNR - SNR^{1 - \alpha}}}{2\mathsf{SNR}^{1-\alpha} + 4}\right)\\
\equiv & 0 \leq 8 + (\mathsf{ 3SNR + SNR^{1-\alpha}} - \mathsf{2SNR^{3
-4\alpha} - 4SNR^{2 - 3\alpha} })\\
\equiv & 0 \leq 4 + (\mathsf{ 2(SNR - SNR^{3-4\alpha})+ SNR^{1-\alpha} + \underbrace{(\mathsf{SNR - 4SNR^{2 - 3\alpha} + 4})} })
\end{eqnarray*}
The last inequality holds because the minimum value of the expression
in under-brace occurs at $\alpha  = \frac{1}{2}, \mathsf{SNR} = 4$, i.e. $0$,
while all other expressions are positive.

In this regime since, $\mathsf{SNR > INR}$, to satisfy \eqref{eq:dec2}
and \eqref{eq:dec3}, it is sufficient to prove
\begin{eqnarray*}
&  R_{2c}  \leq  \log\left(1 +
\frac{\lambda_{c}\mathsf{INR}}{\lambda_p\mathsf{(SNR + INR) +
1}}\right) \\
\equiv & \log(1 + \mathsf{SNR}^{2\alpha - 1}) - \log(3) \leq \log(1 +
\frac{\mathsf{SNR^\alpha - 1 }}{2\mathsf{SNR}^{1-\alpha} + 4})\\
\equiv & 0 \leq 5 + 4\mathsf{(SNR^{1 - \alpha} - SNR^{2\alpha - 1}) +
SNR^{\alpha}}
\end{eqnarray*}
It can be easily seen that the RHS in last inequality is non-negative
for $\alpha \leq \frac{2}{3}$.

To satisfy the inequalities \eqref{eq:dec4}, \eqref{eq:dec5} and
\eqref{eq:dec6}, it is sufficient to prove
\begin{eqnarray*}
& R_{2c} + R_{1r} \leq  \log\left(1 +
\frac{\lambda_{r}\mathsf{SNR} + \lambda_c
\mathsf{INR}}{\lambda_p\mathsf{(SNR + INR) + 1}}\right) \\
& \equiv \log\left(1 + \mathsf{SNR}^{2-3\alpha}\right) + \log(1 + \mathsf{SNR}^{2\alpha - 1}) - \log(9) \leq  \log\left(1 +
\frac{\mathsf{SNR + SNR^\alpha - SNR^{1 -\alpha} - 1 }}{ 2\mathsf{SNR}^{1-\alpha} + 4}\right) \\
\equiv & 0 \leq 12 + \mathsf{2(SNR -  SNR^{2 - 2\alpha}) + 2(SNR - SNR^{3 -4\alpha})} \\
& + \mathsf{(SNR -  SNR^{2\alpha - 1})  + 4(SNR^\alpha - SNR^{2-3\alpha}) + 4(SNR^\alpha - SNR^{2\alpha -1})} + \underbrace{\mathsf{(4SNR - 13SNR^{1 -\alpha} + 11)}}
\end{eqnarray*}
The expression in the under-brace is minimum for $\alpha = \frac{1}{2},
\mathsf{SNR} = (\frac{13}{8})^2$. All the other terms are trivially non-negative.

The final inequality of the 3-user MAC \eqref{eq:dec7} is
\begin{eqnarray*}
  & R_{1r} +R_{1c} + R_{2c} \leq \log\left(1 +
\frac{\lambda_r\mathsf{INR} + \lambda_{c}(\mathsf{SNR} +
\mathsf{INR})}{\lambda_p\mathsf{(SNR + INR) + 1}}\right)\\ \equiv &
\log\left(1 + \mathsf{SNR}^{2-3\alpha}\right) + 2\log(1 +
\mathsf{SNR}^{2\alpha - 1}) -\log(27) \leq \log(1 +
\frac{0.5\mathsf{(1 - SNR^{-\alpha})(SNR +
2SNR^\alpha)}}{\mathsf{SNR^{1 -\alpha} + 2}}) \\ \equiv &  (1 +
\mathsf{SNR}^{2-3\alpha})(1 + \mathsf{SNR}^{2\alpha - 1})^2 \leq 13.5(
\mathsf{1 + SNR^\alpha}) \\  \equiv & 0 \leq 12.5 + \mathsf{(SNR^\alpha
- SNR^{4\alpha -2}) + 2(SNR^\alpha - SNR^{2\alpha -1}) } + \\
 & \mathsf{(SNR^\alpha - SNR^{2 -3\alpha}) + 2(SNR^\alpha - SNR^{1 -
\alpha}) + 6.5SNR^\alpha }
\end{eqnarray*}
Since $\alpha \in \left[\frac{1}{2}, \frac{2}{3} \right)$, each of the
sub-expressions are positive.

Now, we consider the 2-user MAC (decoding constraints at the first
transmitter), i.e satisfying \eqref{eq:2mac}

\begin{eqnarray*}
& R_{2r} \leq \log\left(1 +
\frac{\lambda_r\mathsf{INR}}{\lambda_p\mathsf{INR} + 1}\right) \\
\equiv & \log(1 + \mathsf{SNR}^{2 -3\alpha}) -\log(4) \leq \log(3 +
\mathsf{SNR}^\alpha ) -log(4) \\ \equiv & 0 \leq 2
\end{eqnarray*}

The decoding constraint for rate $R_{2c}$ \eqref{eq:2mac2} is
\begin{eqnarray*}
& R_{2c} \leq \log\left(1 +
\frac{\lambda_c\mathsf{INR}}{\lambda_p\mathsf{INR} + 1}\right) \\
\equiv & \log(1 + \mathsf{SNR}^{2\alpha - 1}) -\log(4) \leq \log(3 +
\mathsf{SNR}^\alpha ) -log(4) \\ \equiv & 0 \leq 2 + \mathsf{SNR^\alpha - SNR^{2\alpha -1}}
\end{eqnarray*}

The final constraint is the sum-rate decoding constraint
\eqref{eq:2mac3} is
\begin{eqnarray*}
& R_{2r} + R_{2c} \leq \log\left(1 + \frac{(\lambda_r +
\lambda_c)\mathsf{INR}}{\lambda_p \mathsf{INR} + 1}\right) \\
\equiv & \log(1 + \mathsf{SNR^{2\alpha - 1}})(1 + \mathsf{SNR^{2 -
3\alpha}}) - \log(16) \leq \log(1 + \mathsf{SNR^\alpha}) - \log(2) \\
\equiv & 0 \leq 7 + 4\mathsf{SNR^\alpha + (SNR^\alpha - SNR^{1 -\alpha})} + \\& \mathsf{(SNR^\alpha - SNR^{2\alpha -1}) + (SNR^\alpha - SNR^{2 - 3\alpha})}
\end{eqnarray*}  \\
All the terms in the RHS of the last expression are positive.

\paragraph{$\alpha \in \left[\frac{2}{3}, 1\right]$} In this regime, the rate tuple described by\eqref{rate:2r1r2-r1r2_3} is achievable without feedback. Thus, the decoding constraints of two 2-user MAC apply. Since $\mathsf{SNR \geq INR}$, the following constraints need to be satisfied
\begin{eqnarray*}
& R_{1c} \leq \log\left( 1 +
\frac{\lambda_c\mathsf{SNR^\alpha}}{\lambda_p \mathsf{SNR +
SNR^\alpha} + 1} \right) \\
 \equiv & \log\left( \frac{\mathsf{SNR}^{2\alpha -1}}{3} \right) \leq \log\left( \frac{\mathsf{SNR}^{1 - \alpha} + \mathsf{SNR}^\alpha + 1}{\mathsf{SNR}^{1 - \alpha} + 2} \right) \\
 \equiv & 0 \leq \mathsf{SNR}^{1 - \alpha} + 1 + 2\frac{\mathsf{SNR}^{2\alpha -1} - \mathsf{SNR}^\alpha}{3}
\end{eqnarray*}
and
\begin{eqnarray*}
& R_{2c} \leq \log\left( 1 +
\frac{\lambda_c\mathsf{SNR^\alpha}}{\lambda_p \mathsf{SNR +
SNR^\alpha} + 1} \right) \\
\equiv & \log\left( \frac{2 \mathsf{SNR}^{1 - \alpha}}{3} \right) \leq \log\left( \frac{\mathsf{SNR}^{1 - \alpha} + \mathsf{SNR}^\alpha + 1}{\mathsf{SNR}^{1 - \alpha} + 2} \right) \\
\equiv & 0 \leq 1+ \frac{1}{3}( \mathsf{SNR}^\alpha - \mathsf{SNR}^{1 - \alpha}) + \frac{2}{3}( \mathsf{SNR}^\alpha - \mathsf{SNR}^{2 - 2\alpha})
\end{eqnarray*}
and finally the bound on the sum-rate
\begin{eqnarray*}
& R_{1c} + R_{2c} \leq \log\left( 1 +
\frac{\lambda_c\mathsf{SNR^\alpha + \mathsf{SNR}}}{\lambda_p \mathsf{SNR +
SNR^\alpha} + 1} \right) \\
\equiv & \log(\mathsf{SNR}^\alpha) - \log(4.5) \leq  \log\left(\frac{\mathsf{SNR} + \mathsf{SNR}^\alpha + 1}{\mathsf{SNR}^{1 - \alpha} +2} \right) \\
 \equiv & \mathsf{SNR} + 2 \mathsf{SNR}^\alpha  \leq 4.5(\mathsf{SNR} + \mathsf{SNR}^\alpha) + 4.5 \equiv 0 \leq 3.5\mathsf{SNR} + 2.5 \mathsf{SNR}^\alpha + 4.5.
\end{eqnarray*}
All the three inequalities can be easily seen to be true.

\subsubsection{Corner point formed by the intersection of \underline{$2R_1 + R_2$ and $R_1$}}\label{cpt3}

\paragraph{$\alpha \in \left[0,\frac{1}{2}\right)$} In this regime, the 
corner point \eqref{rate:2r1r2-r1_1} is achievable without
feedback. Each user treats the message of the other user as noise. The
constraints therefore are
\begin{eqnarray*}
& R_1 \leq \log \left(1 + \frac{\mathsf{SNR}}{2}\right) \\
\equiv &\log(\mathsf{SNR}) - 1 \leq \log \left(1 + \frac{\mathsf{SNR}}{2}\right) \equiv  0 \leq 1
\end{eqnarray*}
and
\begin{eqnarray*}
& R_2 \leq \log\left(1 + \frac{\mathsf{SNR}^{1 - \alpha}}{\mathsf{SNR}^\alpha  + 1}\right) \\
\equiv & \log (\mathsf{SNR}^{1 - 2 \alpha }) - 1 \leq \log\left(1 + \frac{\mathsf{SNR}^{1 - \alpha}}{\mathsf{SNR}^\alpha  + 1}\right) \\
\equiv & 0 \leq 2 + (\mathsf{SNR}^{1 -\alpha} - \mathsf{SNR}^{1 - 2\alpha})
\end{eqnarray*}
Both the inequalities are true for all values of $\mathsf{SNR} > 0$.

\paragraph{$\alpha \in \left[\frac{1}{2}, 1 \right]$} The feasibility of the corner point is triivial.

Now, the feasibility of decoding for $\alpha \in (1,\infty)$ is
proved.
\subsubsection{Corner point formed by the intersection of \underline{$R_1 + R_2$ and $R_1$, $\alpha > 1$}} \label{cpt4}

\paragraph{$\alpha \in (1,2)$} In this case, there are two 2-user MACs and since
$\mathsf{INR}> \mathsf{SNR}$, we list the three tight constraints
\begin{eqnarray*}
R_{1c} \leq \log(1 + \mathsf{SNR}) \equiv \log(\mathsf{SNR}) \leq \log(1 + \mathsf{SNR})
\end{eqnarray*}
the constraint on $R_{2c}$
\begin{eqnarray*}
& R_{2c} \leq \log(1 + \mathsf{SNR}) \equiv \log(\mathsf{SNR}^{\alpha - 1}) \leq \log(1 + \mathsf{SNR}) \\
\equiv & 0 \leq 1 + \mathsf{SNR} - \mathsf{SNR}^{\alpha - 1}
\end{eqnarray*}
and finally the sum-rate constraint
\begin{eqnarray*}
& R_{1c} + R_{2c} \leq \log(1 + \mathsf{SNR} + \mathsf{SNR}^\alpha) \\
\equiv &\log(\mathsf{SNR}^\alpha) \leq \log(1 + \mathsf{SNR} + \mathsf{SNR}^\alpha)
\end{eqnarray*}
Since $\alpha < 2$, all the three inequalities hold.

\paragraph{$\alpha \in [2, \infty)$}  Here we have a 3-user MAC at both the receivers and due
to symmetry feasibility at one of them implies the feasibility at the
other. Without loss of generality, decoding constraints at
$\mathsf{D_1}$ are checked. Noting that $\mathsf{INR} \ge
\mathsf{SNR}^2$, only the tight constraints are listed.
\begin{eqnarray*}
& R_{2r} \leq \log( 1 + \frac{\mathsf{SNR}^{\alpha -1}}{2}) \\
\equiv & \log(\mathsf{SNR}^{\alpha - 2}) - \log(2) \leq \log( 1 + \frac{\mathsf{SNR}^{\alpha -1}}{2}) \\
\equiv & 0 \leq 2 + \mathsf{SNR}^{\alpha -1} - \mathsf{SNR}^{\alpha - 2}
\end{eqnarray*}
 For  $R_{1c}$,
\begin{eqnarray*}
& R_{1c} \leq \log(1 + \mathsf{SNR} (1 - \frac{\mathsf{SNR}^{-1}}{2})) \\
\equiv & \log(\mathsf{SNR}) - \log(2) \leq \log(0.5 + \mathsf{SNR}) \equiv 0 \leq 1 + \mathsf{SNR}
\end{eqnarray*}
and it trivially holds. The decoding of $R_{2c}$ follows from that of $R_{1c}$.
The tight pairwise sum-rate constraints are
\begin{eqnarray*}
& R_{2r} + R_{1c}  \leq \log\left(1 + \frac{\mathsf{SNR}^{\alpha - 1}}{2} + \mathsf{SNR} (1 - \frac{\mathsf{SNR}^{-1}}{2})\right) \\
\equiv & \log(\mathsf{SNR}^{\alpha -1}) - 2 \leq \log(\frac{1}{2} +  \frac{\mathsf{SNR}^{\alpha - 1}}{2} + \mathsf{SNR} ) \\
\equiv & 0 \leq 2 + \mathsf{SNR} + \mathsf{SNR}^{\alpha - 1}
\end{eqnarray*}
and
\begin{eqnarray*}
& R_{1c} + R_{2c} \leq \log\left(1 + (\mathsf{SNR}
+ \mathsf{SNR}^\alpha)(1 - \frac{\mathsf{SNR}^{-1}}{2}) \right) \\
\equiv & \log(\mathsf{SNR}^2) - 2 \leq \log\left(\frac{1}{2} + \mathsf{SNR} + \mathsf{SNR}^\alpha - \frac{\mathsf{SNR}^{\alpha -1}}{2} \right)\\
\equiv & 0 \leq 2 + 4\mathsf{SNR} + 2 (\mathsf{SNR}^\alpha - \mathsf{SNR}^{\alpha -1}) + (\mathsf{SNR}^\alpha - \mathsf{SNR}^2) + \mathsf{SNR}^\alpha.
\end{eqnarray*}
All the terms on RHS are non-negative since $\alpha \ge 2$.  Finally,
the constraint on the total sum-rate
\begin{eqnarray*}
& R_{1c} + R_{2c} + R_{2r} \leq \log\left(1 + (\mathsf{SNR}
+ \mathsf{SNR}^\alpha)(1 - \frac{\mathsf{SNR}^{-1}}{2})
+ \frac{\mathsf{SNR}^{\alpha -1}}{2}\right)\\
\equiv & \log(\mathsf{SNR}^\alpha) - 3 \leq \log(0.5 + \mathsf{SNR} + \mathsf{SNR}^\alpha - \frac{\mathsf{SNR}^{\alpha - 1}}{2} + \frac{\mathsf{SNR}^{\alpha -1}}{2}) \\
\equiv & 0 \leq 4 + 4 (\mathsf{SNR}^\alpha - \mathsf{SNR}^{\alpha - 1}) + 3\mathsf{SNR}^\alpha + 4\mathsf{SNR}^{\alpha -1}
\end{eqnarray*}
All the terms in the RHS of the above expression are non-negative.

\subsubsection{Corner point formed by the intersection of \underline{$R_2$ and $R_1 + R_2$, $\alpha > 1$}} \label{cpt5}

There is a single decoding constraint on the rate $R_{1r} = R_{2r}$
\begin{equation}
R_{1r} \leq \log(1 + \mathsf{SNR}^\alpha) \equiv \log(1 + \mathsf{SNR}^\alpha) \leq \log(1 + \mathsf{SNR}^\alpha).
\end{equation}
