# Supplementary material for: Capacity of All Nine Models of Channel Output Feedback for the Two-user Interference Channel
Source: arXiv:1104.4805 source file (2013-01-25)
Supplement: Supplementary file 5 [file table.tex]

\subsection{Achievable rate pairs for the Gaussian channel}
\subsubsection{Achievability for $(1000)$ Feedback Model}
\label{apga}
\begin{table}[ht] \caption{Power allocation for the private, common and relay messages}
\label{table:lambdas}
\centering
\begin{tabular}{ |c|l|c|c |c|c|c|c|}
\hline %
%\multicolumn {2}{|c|}{Sample} & Roughness $R_a $\\
Corner Point  & $\alpha$& $\lambda_{1p}$ & $\lambda_{2p}$ &$\lambda_{1c}$ & $\lambda_{2c}$ & $\lambda_{1r}$ & $\lambda_{2r}$\\\hline %
& $[0,1/2)$ & 1 & $\min(1, 1/{\sf INR})$ & 0  & 0 & 0 & 0 \\ \cline{2-8}
$\mathcal{P}_{\rm A}$  & $[1/2, 1]$ & 1 & 0 & 0 & 0 & 0 & 0\\ \hline
 & $(1,2]$ & 0 & 0  & $\frac{\sf INR}{\sf SNR^2}$ & 1 & 0 & 0\\ \cline{2-8}
$\mathcal{P}_{\rm B}$ & $(2,\infty$) & 0 & 0 & $1/2$& $1/2$ & $1/2$ & $1/2$ \\ \hline
 & $[0, 1/2)$ & $\min(1,1/{\sf INR})$ & $\min(1,1/{\sf INR})$ & 0 & 0 & $1 - \lambda_{1p}$ & $1 - \lambda_{2p}$ \\\cline {2 -8}
$\mathcal{P}_{\rm C}$ & $[1/2,2/3)$ & $\min(1,1/{\sf INR})$ & $\min(1,1/{\sf INR})$ & $\frac{(1 - \lambda_{1p})}{2}$ & $\frac{(1 - \lambda_{2p})}{2}$ & $\frac{(1 - \lambda_{1p})}{2}$ & $\frac{(1 - \lambda_{2p})}{2}$ \\ \cline{2-8}
& $[2/3,1]$ & $\min(1,1/{\sf INR})$ & $\min(1,1/{\sf INR})$ & 1 - $\lambda_{1p}$ & 1 - $\lambda_{2p}$ & 0 & 0\\ \hline
 & $[0,1]$ & $\min(1,1/{\sf INR})$& $\min(1,1/{\sf INR})$ & 0 & 0 & $1 - \lambda_{1p}$& $1 - \lambda_{2p}$\\ \cline {2 -8}
$\mathcal{P}_{\rm D}$ & $(1,\infty)$ & 0 & 0 & 0 & 0 & 1  &  1 \\\hline
\end{tabular}

\end{table}

\begin{table}[ht]\caption{Rate allocation to the private, common and relay messages}
\label{table:rates}
\centering
\begin{tabular}{ |c|l|c|c |c|c|c|}
\hline %
%\multicolumn {2}{|c|}{Sample} & Roughness $R_a $\\
Corner Point & $\alpha$& $R_{1p}$ & $R_{2p}$ &$R_{1c}$ & $R_{2c}$ & $R_{2r}$ \\\hline %
 & $[0,1/2)$ & $\log({\sf SNR}/{2})$ & $\log({\sf SNR}/{\sf 2 INR^2})$ & 0  & 0 & 0  \\ \cline{2-7}
$\mathcal{P}_{\rm A}$  & $[1/2, 1]$ & $\log(1 + {\sf SNR})$ & 0 & 0 & 0 & 0 \\ \hline
 & $(1,2]$ & 0 & 0  & $\log(1 + \frac{\sf INR}{\sf SNR})$ & $\log({\sf SNR})$ & 0 \\ \cline{2-7}
$\mathcal{P}_{\rm B}$ & (2,$\infty$) & 0 & 0 & $\log({\sf SNR}) -1$& $\log({\sf SNR})  - 1$ & $\log({\sf INR}/{\sf SNR^2}) - 1$ \\ \hline
  & $[0, 1/2)$ & $\log(1 + {\sf SNR}/{\sf 2INR} )$& $R_{1p}$ & 0 & 0 & $\log({\sf INR}/{3})$ \\\cline {2 -7}
& & & & & & \\
$\mathcal{P}_{\rm C}$ & $[1/2,2/3)$ & $\log(1 + \frac{\sf SNR}{\sf 2INR})$ & $R_{1p}$ & $\log(1 + \frac{\sf INR^2}{\sf SNR}) -2$  & $R_{1c}$ & $\log(\frac{1 + {\sf SNR^2}/{\sf2 INR^3}}{4})$  \\
 & & & & & & \\ \cline{2-7}
 & $[2/3,1]$ & $\log(1 + {\sf SNR}/{\sf 2INR})$ & $R_{1p}$  & $\log({\sf INR^2}/{\sf 3SNR})$ & $\log({\sf 2SNR}/{\sf 3INR})$ & 0 \\ \hline
 & $[0,1]$ & $\log(1 + \frac{\sf SNR}{2 {\sf INR} })$& $R_{1p}$ & 0 & 0 & $\log(\frac{{\sf INR}}{3})$ \\ \cline {2 -7}
$\mathcal{P}_{\rm D}$ & $(1,\infty)$ & 0 & 0  & 0 & 0 & $\log(1 + {\sf INR})$  \\\hline
\end{tabular}
\end{table}

The rate and power allocation to achieve within a constant number of
bits of all non-trivial corner points for the feedback model $(1000)$
are given in Tables~\ref{table:lambdas} and \ref{table:rates}. The
achievable rates for ${\sf T}_1$-${\sf D}_1$ user pair is $R_1 =
R_{1p} + R_{1c}$ and ${\sf T}_2$-${\sf D}_2$ user pair is $R_2 =
R_{2p} + R_{2c} + R_{2r}$. The points $\mathcal{P}_{\rm A},
\mathcal{P}_{\rm B}, \mathcal{P}_{\rm C}$ and $\mathcal{P}_{\rm D}$
describe four different achievable rate pairs $(R_1,R_2)$ using $(1000)$ feedback model.

\subsubsection{Achievability for $(0010)$ Feedback Model}
\label{sec:(0010)_l}
Here we show the rate and power allocation for achieving a rate pair
within constant number of bits from $\overline{\mathcal{K}}_{\rm B}$
in $(0010)$ feedback model in the weak interference regime. At ${\sf
  T}_1$, all the power is used to transmit $X_{1i}$. The power
allocation at ${\sf T}_2$ is
\begin{eqnarray}
  \lambda_{2,d} = \frac{\sf INR}{2\mathsf{SNR}}, \text{ }\lambda_{2,nd} = \frac{1}{2\mathsf{INR}^2}, \text{ }\lambda_{2',d} = 1 - \lambda_{2,d} - \lambda_{2,nd}\text{ when } {\alpha \leq \frac{1}{2}} \label{eq:(0010)_l1}\\
  \lambda_{2,d} = \frac{1}{\sf INR}, \text{ }\lambda_{2,nd} = 0, \text{ }\lambda_{2',d} = 1 - \lambda_{2,d} \text{ when } {\alpha} \geq \frac{1}{2} \label{eq:(0010)_l2}
\end{eqnarray}
while the rate allocation is
\begin{eqnarray}
  R_1 & = &\log\left(1 + \frac{\sf SNR}{2}\right), \text{ }R_{2,d} = \min\left\{\log\left(\frac{\sf INR}{2}\right),\log\left(\frac{\sf SNR}{2\mathsf{INR}}\right)\right\} \label{eq:(0010)_r1}\\
R_{2,nd} & = &\log\left(\frac{\sf SNR}{{\sf2 INR}^2}\right) \text{ when } {\alpha} \leq \frac{1}{2}, \text{ } 0 \text{ otherwise} \label{eq:(0010)_r2}
\end{eqnarray}

 %% Note that,
%% whenever $R_{2r} = 0$, feedback is not necessary.
