# Supplementary material for: Capacity of All Nine Models of Channel Output Feedback for the Two-user Interference Channel
Source: arXiv:1104.4805 source file (2013-01-25)
Supplement: Supplementary file 8 [file alt_cpt.tex]

\paragraph{Corner point: Intersection of $R_1$ and $R_1 + R_2$} Again
the regime of $\alpha \in (0, \infty)$ can be divided into parts.

$\alpha \in (1, 2)$

$\alpha \in [2, \infty)$ To achieve the corner point in this regime,
we adopt the feedback strategy \textbf{(mention described above)}. The
power sharing is given as follows
\begin{equation}
\lambda_{ur} = \min \left(1,\frac{1}{\mathsf{SNR}}\right);
\lambda_{uc} = 1 - \lambda_{ur}.
\end{equation}
The achievable rate for the this choice of power are
\begin{eqnarray}
R_{ur} = \log(\frac{\mathsf{INR}^2}{\mathsf{SNR}})
R_{uc} = {\log (\mathsf{SNR}) - 1}^+ \nonumber \\
\end{eqnarray}

The rate $R_{1r}$
\begin{eqnarray*}
& R_{1r} \leq \log\left(1 + SNR^{\alpha -1}\right) \\
\equiv & \mathsf{SNR}^{\alpha  - 2} \leq 1 + SNR^{\alpha -1} 
\end{eqnarray*}
The individual rate $R_{2c}$ has a tighter constraint than $R_{1c}$
\begin{eqnarray*}
& R_{2c} \leq \log\left(\mathsf{SNR}\right) \\
\equiv & \log\left(\mathsf{SNR}\right) -1 \leq \log\left(\mathsf{SNR}\right)
\end{eqnarray*}
The sum rate constraints are
\begin{eqnarray*}
R_{1c} + R_{2c} \leq \log (1 + \mathsf{SNR + SNR^\alpha - SNR^{-\alpha} - SNR^{\alpha -2} + 1 ) \\
\equiv 0 \leq  1 + \mathsf{SNR + (SNR^\alpha - SNR^2) - SNR^{-\alpha} - SNR^{\alpha -2} + 1 
\end{eqnarray*}
