# Supplementary material for: Capacity of All Nine Models of Channel Output Feedback for the Two-user Interference Channel
Source: arXiv:1104.4805 source file (2013-01-25)
Supplement: Supplementary file 9 [file apc-shrunk.tex]

\subsection{Gap to Capacity}
\label{gap}
In this section, we show that the gap between the corner points of the
outer bound and the achievable scheme is at most 6 bits/Hz for the
$(1000)$ feedback model. The gap for $(1\times\times 1)$ model has
been shown to be no more than 3.59 bits/Hz. The gap between outer
bound and achievable rate region for the $(1100)$ and $(1110)$ too is
3.59 bits/Hz.

The outer bounds on $R_1 + R_2$ (Theorem \ref{th:sum-capg}) and $2R_1
+ R_2$ (Theorem \ref{th:sum-capg2}) are a function of correlation
$\rho$ between the transmitted symbols $X_1$ and $X_2$. By plugging in
$\rho$ that maximizes the expressions of outer-bounds described by
Theorem \ref{th:sum-capg} and Theorem \ref{th:sum-capg2}, outer bounds
for rates $R_1 + R_2$ for $(1\times \times \text{ }0)$ feedback model
and $2R_1 + R_2$ for $(1000)$ feedback model are obtained. The bounds
on rates $R_1 + R_2$ and $2R_1 + R_2$ together with the bounds on
$R_1$ and $R_2$, form the outer bound of the capacity region of for
different regimes of interference (different values of $\alpha$). The
outerbound of the capacity region will be denoted by
$\overline{\mathcal{C}}$. Points on the boundary are denoted by
$(\overline{C}_1, \overline{C}_2)$, such that $(\overline{C}_1,
\overline{C}_2) \in \overline{\mathcal{C}}$. The achievable rate tuple
are denoted by $(R_1, R_2)$. Since the achievability described
differently for two broad regimes of interference, i.e. $\alpha \in
[0,1] $ and $\alpha \in (1, \infty)$.  All the corners point of
interest are listed below for whiich the achievability is described in
Section \ref{subsec:onelink_a_l}.

\subsubsection{Corner point formed by intersection \underline{$R_2$ and $R_1 +R_2$}} 
\label{para:r2-r1r2_l} \text{ }

\paragraph{$\alpha \in [0,1]$:} This corner point is achievable within constant gap
from achievable rates described in \eqref{rate:r2-r1r2}.
\noindent The outer bound on rate $R_2$  is $ \overline{C}_2 = \log(1 +
\mathsf{SNR +  INR})$. The gap of the achievable rate from the outer bound is  
\begin{eqnarray*}
\overline{C}_2 - R_2 & \leq & \log(1 + \mathsf{SNR} + \mathsf{INR}) - \log\left( 1 + \frac{\mathsf{SNR}}{2\mathsf{INR}}\right) - \log(\mathsf{INR}) + \log(3) \\ 
& = & \log\left( \frac{1 + \mathsf{INR} + \mathsf{SNR}}{2\mathsf{INR}
+ \mathsf{SNR}}\right) + \log(2) + \log(3)\\ & \leq & 1 + \log(3)
\end{eqnarray*} The corresponding gap from the $\overline{C}_1$ is
\begin{eqnarray*}
\overline{C_1} - R_1 & \leq & [\log \left( 1 +
\frac{ \mathsf{SNR}}{1 + \mathsf{INR}}\right) + \log (1 + \mathsf{SNR + INR} +
2\sqrt{\mathsf{SNR. INR}} )  -  \log(1 + \mathsf{SNR + INR})] - \log\left(1 + \frac{\mathsf{SNR}}{2\mathsf{INR}} \right) \\
& \leq & \log\left(\frac{1 + \mathsf{INR} + \mathsf{SNR}}{2\mathsf{INR} + \mathsf{SNR}}\right) + \log\left(\frac{\mathsf{INR}}{\mathsf{INR} + 1}\right) + \log\left(1 + \frac{2\sqrt{\mathsf{SNR}.\mathsf{INR}}}{1 + \mathsf{SNR} + \mathsf{INR}}\right)  + \log(2)\\
& \leq &  \log(3) + 1 
\end{eqnarray*}

\subsubsection{Corner point formed by intersection \underline{$2R_1 + R_2$ and $R_1 + R_2$}} 
\label{para:2r1r2-r1r2} \text{ }
Proceeding on the lines of the achievability scheme, we split the gap
computation into three different regimes. 

\paragraph{$\alpha \in \left[0,\frac{1}{2}\right)$:} The distance of the outer
bound from the achievable rate $R_2$ obtained in \eqref{rate:r2-r1r2}
\begin{eqnarray*}
\overline{C}_2 - R_2 & \leq & [\log \left( 1 +
\frac{\mathsf{SNR}}{1 + \mathsf{INR}}\right) + \log\left(1 + \mathsf{SNR} + \mathsf{INR} + 2\sqrt{\mathsf{SNR}.\mathsf{INR}}\right) - \log\left(1 + \mathsf{INR} +  \frac{\mathsf{SNR} -2\mathsf{INR} + 2\sqrt{\mathsf{SNR}.\mathsf{INR}}}{1 + \mathsf{INR}}\right)] \\
&& - [\log\left(1 + \frac{\mathsf{SNR}}{2\mathsf{INR}}\right) + \log(\mathsf{INR}) - \log(3)] \\
& \leq & \log\left(\frac{1 + \mathsf{SNR} + \mathsf{INR}}{2\mathsf{INR} + \mathsf{SNR}}\right) +  \log\left(\frac{1 + \mathsf{SNR} + \mathsf{INR} + 2\sqrt{\mathsf{SNR}.\mathsf{INR}}}{1 + \mathsf{SNR} + \mathsf{INR}^2 + 2\sqrt{\mathsf{SNR}.\mathsf{INR}}}\right)  + \log(2) + \log(3) \\
&\leq & \log(2) + \log(3) = 1 + \log(3).
\end{eqnarray*}
The corresponding gap for the achievable rate $R_1$
\begin{eqnarray*}
\overline{C}_1 - R_1 & \leq &\log\left(1 + \mathsf{INR} + \frac{\mathsf{SNR - (1 + \rho^2)INR + 2\rho\sqrt{SNR.INR}}}{\mathsf{INR + 1}}\right) -\log\left( 1 + \frac{\mathsf{SNR}}{2\mathsf{INR}}\right)  \\
& \leq & \log\left(\frac{\mathsf{INR} + \mathsf{INR}^3 + \mathsf{SNR}.\mathsf{INR} + 2\mathsf{INR}\sqrt{\mathsf{SNR}.\mathsf{INR}}}{\mathsf{SNR}.(\mathsf{INR} + 1)}\right) +  \log(2) \\
& \leq &  \log\left(\frac{\mathsf{INR} + \mathsf{SNR}.\mathsf{INR}}{\mathsf{SNR} + \mathsf{SNR}.\mathsf{INR}}+ \frac{\mathsf{INR}}{\mathsf{INR} +1 }\frac{\mathsf{INR}^2 +  2\sqrt{\mathsf{SNR}.\mathsf{INR}}}{\mathsf{SNR}}\right) + 1 \\
& \leq & \log(4) + 1 = 3.
\end{eqnarray*}

\paragraph{${\alpha \in \left[0.5,\frac{2}{3}\right)}$} The achievable rate is
described \eqref{rate:2r1r2-r1r2_2} in and the distance of $R_1$ from
the outer bound is bounded as follows
\begin{eqnarray*}
\overline{C}_2 - R_2 & \leq &  \log \left( 1 +
\frac{ \mathsf{SNR}}{1 + \mathsf{INR}}\right) + \log (1 + \mathsf{SNR + INR} +
2\sqrt{\mathsf{SNR. INR}} ) - \log\left(1 +
\mathsf{INR} + \frac{\mathsf{SNR - 2INR + 2\sqrt{SNR.INR} }}{\mathsf{INR + 1}}\right) \\
 && - [\log\left(1 + \frac{\mathsf{SNR}}{\mathsf{2INR}}\right) + \log\left(1 + \frac{\mathsf{INR}^2}{\mathsf{SNR}}\right) + \log\left(1 + \frac{\mathsf{SNR}^2}{\mathsf{INR}^3}\right)-2\log(4)] \\
& \leq  & \log\left(\frac{1 + \mathsf{INR} + \mathsf{SNR} + 2\sqrt{\mathsf{SNR}.\mathsf{INR}}}{1 + \mathsf{INR}^2 + \mathsf{SNR} + 2\sqrt{\mathsf{SNR}.\mathsf{INR}}}.\frac{\mathsf{SNR}.\mathsf{INR}^2}{\mathsf{SNR}^2 + \mathsf{INR}^3}\right) + \log(2) + 4 \leq \log(2) + 5  =6
\end{eqnarray*}
and the gap from the outer bound for the rate $R_1$ is  
\begin{eqnarray*}
\overline{C}_1 - R_1 & = &[\log\left(1 + \mathsf{INR} + \frac{\mathsf{SNR - 2INR + 2\sqrt{SNR.INR}}}{\mathsf{INR + 1}}\right)] - [\log\left(1 + \frac{\mathsf{SNR}}{2\mathsf{INR}}\right) + \log\left(1 + \frac{\mathsf{INR}^2}{\mathsf{SNR}}\right) -\log(4)] \\
& \leq &\log\left(\frac{1 + \mathsf{INR} + \mathsf{SNR} + 2\sqrt{\mathsf{SNR}.\mathsf{INR}}}{\mathsf{INR} + 1}\right) - [\log\left(1 + \frac{\mathsf{SNR}}{2\mathsf{INR}}\right) + \log\left(\frac{\mathsf{INR}^2}{\mathsf{SNR}}\right) ] +\log(4) \\
& \leq &  \log\left(\frac{1 + \mathsf{INR} + \mathsf{SNR} + 2\sqrt{\mathsf{SNR}.\mathsf{INR}}}{\mathsf{INR} + 1}.\frac{\mathsf{SNR}}{\mathsf{INR}^2 + \mathsf{INR}.\mathsf{SNR}} \right) + \log(2) + 2 \\
& \leq & \log(1.5) + \log(2) + 2 = 2 + \log(3).
\end{eqnarray*}

\paragraph{${\alpha \in \left[\frac{2}{3}, 1 \right]}$} The achievable rate tuple,
obtained without feedback, is described in
\eqref{rate:2r1r2-r1r2_3}. The gap from the outer bound for the achievable  $R_2$ is
\begin{eqnarray*}
\overline{C}_2 - R_2 & \leq &  \log \left( 1 +
\frac{ \mathsf{SNR}}{1 + \mathsf{INR}}\right) + \log (1 + \mathsf{SNR + INR} +
2\sqrt{\mathsf{SNR. INR}} ) \\ & & - \log\left(1 +
\mathsf{INR} + \frac{\mathsf{SNR - 2INR + 2\sqrt{\mathsf{SNR}.\mathsf{INR}} }}{\mathsf{INR + 1}}\right) - [\log\left(\frac{\mathsf{SNR}}{\mathsf{INR}}\right) + \log\left(1 + \frac{\mathsf{SNR}}{2\mathsf{INR}}\right) - \log(1.5)] \\
& \leq & \log\left(\frac{1 + \mathsf{INR} + \mathsf{SNR}}{2\mathsf{INR} + \mathsf{SNR}}\right) + \log\left(\frac{1 + \mathsf{INR} + \mathsf{SNR} + 2\sqrt{\mathsf{INR}.\mathsf{SNR}}}{1 + \mathsf{INR}^2 + \mathsf{SNR} + 2\sqrt{\mathsf{INR}.\mathsf{SNR}}}.\frac{\mathsf{SNR}}{\mathsf{INR}^2}\right) + \log(2) + \log(1.5) \\
&\leq &  \log\left(\frac{1 + \mathsf{INR} + \mathsf{SNR}}{2\mathsf{INR} + \mathsf{SNR}}\right) + \log\left(\frac{\mathsf{INR}^2 + \mathsf{INR}^3 + \mathsf{SNR}.\mathsf{INR}^2 + 2\sqrt{\mathsf{INR}.\mathsf{SNR}}.\mathsf{INR}^2}{\mathsf{SNR} + \mathsf{SNR}.\mathsf{INR}^2 + \mathsf{SNR}^2 + 2\sqrt{\mathsf{INR}.\mathsf{SNR}}.\mathsf{SNR}}\right) + \log(3) \\
& \leq & \log(4) + \log(3) = 2 + \log(3)
\end{eqnarray*}
and the correponding gap of the outer bound from $R_1$ is given by
\begin{eqnarray*}
\overline{C}_1 - R_1 & \leq & \log\left(1 + \mathsf{INR} + \frac{\mathsf{SNR - 2INR + 2\sqrt{SNR.INR}}}{\mathsf{INR + 1}}\right) \\
& & - [\log \left(1 + \frac{\mathsf{SNR}}{2\mathsf{INR}}\right) - \log\left(
\frac{\mathsf{INR}^2}{\mathsf{SNR}}\right) - \log(3)] \\
& \leq &   \log\left(\frac{1 + \mathsf{INR}^2 + \mathsf{SNR} + 2\sqrt{\mathsf{SNR}.\mathsf{INR}}}{\mathsf{INR}.(\mathsf{INR} + 1)} \right) + \log\left( \frac{\mathsf{SNR}}{\mathsf{SNR} + 2\mathsf{INR}}\right) + \log(2) +\log(3) \\
& \leq & \log\left(1 + \frac{\mathsf{SNR} + 2\sqrt{\mathsf{SNR}.\mathsf{INR}}}{\mathsf{INR}.(\mathsf{INR} + 1)}\right) + \log\left(\frac{\mathsf{SNR}}{\mathsf{SNR} + 2\mathsf{INR}}\right) + 1 + \log(3) \\
& \leq & \log\left(1 + \frac{\mathsf{SNR}^2 + 2\sqrt{\mathsf{SNR}.\mathsf{INR}}.\mathsf{SNR}}{2\mathsf{INR}^3 + \mathsf{SNR}.\mathsf{INR}^2 + \mathsf{SNR}.\mathsf{INR} + 2\mathsf{INR}^2}\right) + 1 + \log(3) \\
& \leq & 2 + \log(3)
\end{eqnarray*}

\subsubsection{Corner point of intersection of \underline{$2R_1 + R_2$ and $R_1$ bounds}}\label{para:2r1r2-r1} \text{ }
It is sufficient to consider only two regimes.

\paragraph{$\alpha \in \left[0, \frac{1}{2}\right)$} This rate tuple
\eqref{rate:2r1r2-r1_1} is achievable without feedback and the gaps from 
the outer bound are given by
\begin{eqnarray*}
\overline{C}_2 - R_2 & \leq &  \log \left( 1 +
\frac{ \mathsf{SNR}}{1 + \mathsf{INR}}\right) + \log (1 + \mathsf{SNR + INR} +
2\sqrt{\mathsf{SNR. INR}} ) + \nonumber \\
&& [\log\left(1 + \mathsf{INR} + \frac{\mathsf{SNR} - 2 \mathsf{INR} + 2\sqrt{\mathsf{SNR.INR} }}{1+
\mathsf{INR}}\right)   - 2\log(1 + \mathsf{SNR})] - [\log\left(\frac{\mathsf{SNR}}{\mathsf{INR}^2}\right) - 1]  \\
&\leq & \log\left(\frac{1 + \mathsf{INR} + \mathsf{SNR}}{1 + \mathsf{SNR}}\right) + \log\left(\frac{1 + \mathsf{INR} + \mathsf{SNR} + 2\sqrt{\mathsf{SNR}.\mathsf{INR}}}{1 + \mathsf{SNR}}\right) + \log\left(\frac{1 + \mathsf{INR}^2 + \mathsf{SNR} + 2\sqrt{\mathsf{SNR}.\mathsf{INR}}}{1 + \mathsf{INR}^2 + 2\mathsf{INR}}\right) \\
& \leq & \log\left(\frac{1 + \mathsf{INR} + \mathsf{SNR}}{1 + \mathsf{SNR}}.\frac{1 + \mathsf{INR}^2 + \mathsf{SNR} +  2\sqrt{\mathsf{SNR}.\mathsf{INR}}}{1 + \mathsf{INR}^2 + \mathsf{SNR}}\right) + \log\left(\frac{1 + \mathsf{INR}^2 + \mathsf{SNR} + 2\sqrt{\mathsf{INR}.\mathsf{SNR}}}{1 + \mathsf{INR}^2 + 2\mathsf{INR}}\frac{\mathsf{INR}^2}{\mathsf{SNR}}\right) +  1  \\
& \leq & \log(4) + \log(3) + 1 = 3 + \log(3)
\end{eqnarray*}
and
\begin{eqnarray*}
\overline{C}_1 - R_1 & \leq& \log(1 + \mathsf{SNR}) - [\log(\mathsf{SNR}) - 1 ] \leq \log\left(\frac{1 + \mathsf{SNR}}{\mathsf{SNR}}\right) + 1 = 2.
\end{eqnarray*}

\paragraph{$\alpha \in \left[\frac{1}{2}, \frac{2}{3}\right)$} The achievable
rates are corresponding distances from the outer bounds are
\begin{eqnarray*}
\overline{C}_2 - R_2 & \leq &   \log \left( 1 +
\frac{ \mathsf{SNR}}{1 + \mathsf{INR}}\right) + \log (1 + \mathsf{SNR + INR} +
2\sqrt{\mathsf{SNR. INR}} ) + \nonumber \\
&& \log\left(1 + \mathsf{INR} + \frac{\mathsf{SNR} - 2 \mathsf{INR} + 2\sqrt{\mathsf{SNR.INR} }}{1+
\mathsf{INR}}\right)   - 2\log(1 + \mathsf{SNR}) \\
&\leq & \log\left(\frac{1 + \mathsf{INR} + \mathsf{SNR}}{1 + \mathsf{SNR}}\right) + \log\left(\frac{1 + \mathsf{INR} + \mathsf{SNR} + 2\sqrt{\mathsf{SNR}.\mathsf{INR}}}{1 + \mathsf{SNR}}\right) + \log\left(\frac{1 + \mathsf{INR}^2 + \mathsf{SNR} + 2\sqrt{\mathsf{SNR}.\mathsf{INR}}}{1 + \mathsf{INR}^2 + 2\mathsf{INR}}\right) \\
& \leq & \log(\frac{1 + \mathsf{INR} + \mathsf{SNR}}{1 + \mathsf{SNR}}.\frac{1 + \mathsf{INR}^2 + \mathsf{SNR} +  2\sqrt{\mathsf{SNR}.\mathsf{INR}}}{1 + \mathsf{INR}^2 + \mathsf{SNR}}) + \log(2) \\
& \leq & \log\left( 1 + \frac{ \mathsf{INR} + 2\sqrt{\mathsf{SNR}.\mathsf{INR}}+ \mathsf{SNR}.\mathsf{INR} + 2\sqrt{\mathsf{SNR}.\mathsf{INR}}.\mathsf{INR} + \mathsf{INR}^3 + 2\sqrt{\mathsf{SNR}.\mathsf{INR}}\mathsf{SNR}}{1 + \mathsf{INR}^2 + 2\mathsf{SNR} + \mathsf{SNR}.\mathsf{INR}^2 + \mathsf{SNR}^2}\right) + \log(2) \\
&\leq  & \log(4) + \log(2) = 3.
\end{eqnarray*}
Both the outer and inner bounds for $R_1$ are $\log(1 + \mathsf{SNR})$ and
thus the gap is 0. The point $(\log(1 + \mathsf{SNR}), 0)$ is
trivially achievable.

Now we list the gap for corner points where $\alpha \in (1, \infty)$. 

\subsubsection{Corner point of intersection of \underline{$R_1$ and $R_1 + R_2$}}\label{para:r1-r_1r_2}\text{ } 
\paragraph{$\alpha \in (1,2)$} The achievability is described in Section \ref{subsec:onelink_a_l}.
The achievable rates \eqref{rate:r1-r1r2_h1} and its gap from the
outer bound is
\begin{eqnarray*}
\overline{C}_2 - R_2 & \leq & [\log\left(1 + \frac{\mathsf{SNR}}{1 + \mathsf{INR}}\right) + \log(1 + \mathsf{SNR} + \mathsf{INR} + 2\sqrt{\mathsf{SNR}.\mathsf{INR}}) - \log(1 + \mathsf{SNR})] - \log\left(\frac{\mathsf{INR}}{\mathsf{SNR}}\right) \\
& \leq & \log(2) + \log\left(\frac{\mathsf{SNR} + \mathsf{SNR}^2 + \mathsf{SNR}.\mathsf{INR} + 2\sqrt{\mathsf{SNR}.\mathsf{INR}}.\mathsf{SNR}}{\mathsf{SNR}.\mathsf{INR} + \mathsf{INR}}\right) \leq \log(2) + \log(4) = 3
\end{eqnarray*}
The gap from the achievable rate $R_1$ is 
\begin{eqnarray*}
\overline{C}_1 - R_1 & \leq & \log(1 + \mathsf{SNR}) - \log(\mathsf{SNR})\\
& \leq & \log(2)  = 1
\end{eqnarray*}

\paragraph{$\alpha \in [2, \infty)$} The achievable rate tuple
  \eqref{rate:r1-r1r2_h2} is achieved with feedback. The outer bound
  on $R_2$ and its gap from the outer bound is
\begin{eqnarray*}
\overline{C}_2 - R_2 & \leq &  [\log(1 + \mathsf{INR} + \mathsf{SNR} + 2\sqrt{\mathsf{INR}.\mathsf{SNR}}) - \log(1 + \mathsf{SNR})] - [\log\left(\frac{\mathsf{INR}}{\mathsf{SNR}}\right) -2] \\
& \leq & \log\left(\frac{\mathsf{SNR} + \mathsf{INR}.\mathsf{SNR} + \mathsf{SNR}^2 + 2\sqrt{\mathsf{INR}.\mathsf{SNR}}}{\mathsf{INR} + \mathsf{INR}.\mathsf{SNR}}\right) + 2 \\
& \leq & \log\left(1 + \frac{\mathsf{SNR}^2 + 2\sqrt{\mathsf{INR}.\mathsf{SNR}}}{\mathsf{INR} + \mathsf{INR}.\mathsf{SNR}}\right) + 2 \\
& \leq & \log(3) + 2 
\end{eqnarray*}
The gap from the outer bound for the achievable rate $R_1$ is 
\begin{eqnarray*}
\overline{C}_1 - R_1 & \leq & \log\left(1 + \mathsf{SNR}\right) - [\log(\mathsf{SNR}) -1] \\
& \leq & \log\left(1 + \frac{1}{\mathsf{SNR}}\right) + 1 \leq \log(2) + 1 =2
\end{eqnarray*}

\subsubsection{Corner point of intersection of \underline{$R_2$ and
    $R_1 + R_2$}} \label{para:r2-r1r2_h}\text{ }  
\paragraph{$\alpha \in (1, \infty)$} The achievability of the corner point is
described in Section \ref{subsec:onelink_a_l} and the achievable
rate-tuple is described by (\ref{rate:r2-r1r2_h}). The gap of the
achievable rate $R_2$ from the outer bound is
\begin{eqnarray*}
  \overline{C}_2 - R_2 &\leq & \log\left(1 + \frac{\mathsf{SNR}}{1 +
    \mathsf{INR}}\right) + \log(1 + \mathsf{INR} + \mathsf{SNR} +
  2\sqrt{\mathsf{INR}.\mathsf{SNR}}) - \log(1 + \mathsf{INR}) \\ &
  \leq & \log(2) + \log\left(1 + \frac{\mathsf{SNR} +
    2\sqrt{\mathsf{SNR}.\mathsf{INR}}}{1 + \mathsf{INR}}\right) \\ &
  \leq & \log(2) + \log(4) = 3.
\end{eqnarray*}
The achievable rate $R_1 = 0$ and the corresponding gap from the outer
bound corner point is 
\begin{eqnarray*}
\overline{C}_1 - R_1 &\leq & \log\left(1 + \frac{\mathsf{SNR}}{1 + \mathsf{INR}}\right) + \log(1 + \mathsf{INR} + \mathsf{SNR} + 2\sqrt{\mathsf{INR}.\mathsf{SNR}}) - \log(1 + \mathsf{INR} + \mathsf{SNR}) \\
& \leq & \log(2) + \log\left(1 + \frac{2\sqrt{\mathsf{SNR}.\mathsf{INR}}}{1 + \mathsf{INR} + \mathsf{SNR}}\right) \\
& \leq & \log(2) + \log(2) = 2
\end{eqnarray*}

\subsubsection{Corner point of intersection of \underline{$R_2$ and
    $R_1 + R_2$}} \text{ }

In the regime where $1 < \alpha < 2$, the rate pairs achieved without any
feedback are shown to be within the constant number of bits from the
corner point of intersection of the outer bound of sum-rate  $R_1 +
R_2$ (Theorem \ref{th:sum-capg}) and rate $R_2$.

\paragraph{$\alpha \in (1,2)$}  In the regime $\alpha \in (1,2)$, the
outer bound for rate $R_1 + R_2$ is due to Theorem \ref{th:sum-capg},
while the outer bound on rate $R_2$ is due to a symmetric version of
Theorem \ref{th:r2}. 
\begin{eqnarray*}
\overline{C}_1 - R_1 & \leq & \log \left(1 + \frac{\mathsf{SNR}}{ 1 +
  \mathsf{INR}}\right) + \log(1 + \mathsf{SNR + INR} +
2\sqrt{\mathsf{SNR.INR}}) - \log(1 + \mathsf{SNR}) - \log\left(1 +
\frac{\mathsf{INR}}{\mathsf{SNR}} \right) \\
 & \leq & \log(2) + \log(2) + \log \left(\frac{\mathsf{SNR} + \mathsf{SNR}^2
  + \mathsf{INR.SNR} +
  2\mathsf{SNR}.\sqrt{\mathsf{SNR}.\mathsf{INR}}}{\mathsf{2SNR + 2SNR^2
    + 2INR + 2INR.SNR }} \right) \leq 2.
\end{eqnarray*}

\begin{eqnarray*}
\overline{C}_2 - R_2 & \leq & \log(1 + \mathsf{SNR})  -
\log(\mathsf{SNR}) \leq  1.
\end{eqnarray*}

\paragraph{$\alpha \in [2, \infty)$}
($\log(1 + \mathsf{SNR})$ , $\log(1 + \mathsf{SNR})$) is a achievable
  rate pair for the regime of $\alpha \geq 2$.
