# Supplementary material for: Capacity of All Nine Models of Channel Output Feedback for the Two-user Interference Channel
Source: arXiv:1104.4805 source file (2013-01-25)
Supplement: Supplementary file 12 [file table2.tex]

\subsection{Achievable rate pairs for the Gaussian channel}
\subsubsection{Achievability for $(1000)$ Feedback Model}
\label{apga}
\begin{table}[t] \caption{Power allocation for the private and common messages}
\label{table:lambdas}
\centering
\begin{tabular}{ |c|l|c|c |c|c|c|}
\hline %
%\multicolumn {2}{|c|}{Sample} & Roughness $R_a $\\
Corner Point  & $\alpha$& $\lambda_{1p}$ & $\lambda_{2p}$ &$\lambda_{1c}$ & $\lambda_{2c}$ & $\lambda_{1r}$ \\\hline %
& $[0,1/2)$ & 1 & $\min(1, 1/{\sf INR})$ & 0  & 0 & 0  \\ \cline{2-7}
$\mathcal{P}_{\rm A}$  & $[1/2, 1]$ & 1 & 0 & 0 & 0 & 0 \\ \hline
 & $(1,2]$ & 0 & 0  & 1 &  1 & 0 \\ \cline{2-7}
$\mathcal{P}_{\rm B}$ & $(2,\infty$) & 0 & 0 & $1 - \frac{1}{\sf SNR}$& $1$ & $\frac{1}{\sf SNR}$  \\ \hline
 & $[0, 1/2)$ & $\min(1,1/{\sf INR})$ & $\min(1,1/{\sf INR})$ & 0 & $1 - \lambda_{1p}$ & $1 - \lambda_{2p}$  \\\cline {2 -7}
$\mathcal{P}_{\rm C}$ & $[1/2,2/3)$ & $\min(1,1/{\sf INR})$ & $\min(1,1/{\sf INR})$ & $\frac{(1 - \lambda_{1p})}{2}$ & $(1 - \lambda_{2p})$ & $\frac{(1 - \lambda_{1p})}{2}$  \\ \cline{2-7}
& $[2/3,1]$ & $\min(1,1/{\sf INR})$ & $\min(1,1/{\sf INR})$ & 1 - $\lambda_{1p}$ & 1 - $\lambda_{2p}$ & 0 \\ \hline
 & $[0,1]$ & $\min(1,1/{\sf INR})$& $\min(1,1/{\sf INR})$ & 0 & $1 - \lambda_{1p}$ & $1 - \lambda_{2p}$   \\ \cline {2-7}
$\mathcal{P}_{\rm D}$ & $(1,\infty)$ & 0 & 0 & 0 &   1  &  1 \\\hline
\end{tabular}

\end{table}

\begin{table}[t]\caption{Rate allocation to the private and common messages}
\label{table:rates}
\centering
\begin{tabular}{ |c|l|c|c |c|c|c|}
\hline %
%\multicolumn {2}{|c|}{Sample} & Roughness $R_a $\\
Corner Point & $\alpha$& $R_{1p}$ & $R_{2p}$ &$R_{1c}$ & $R_{2c}$ \\\hline %
 & $[0,1/2)$ & $\log({\sf SNR}/{2})$ & $\log({\sf SNR}/{\sf 2 INR^2})$ & 0  & 0   \\ \cline{2-6}
$\mathcal{P}_{\rm A}$  & $[1/2, 1]$ & $\log(1 + {\sf SNR})$ & 0 & 0 & 0  \\ \hline
 & $(1,2]$ & 0 & 0  &   $\log({\sf SNR})$ & $\log(1 + \frac{\sf INR}{\sf SNR})$  \\ \cline{2-6}
$\mathcal{P}_{\rm B}$ & (2,$\infty$) & 0 & 0 & $\log({\sf SNR})$& $\log({\sf \frac{INR}{SNR}}) $  \\ \hline
  & $[0, 1/2)$ & $\log(1 + {\sf SNR}/{\sf 2INR} )$& $R_{1p}$ & 0 & $\log({\sf INR}/{3})$  \\\cline {2 -6}
& & & & &  \\
$\mathcal{P}_{\rm C}$ & $[1/2,2/3)$ & $\log(1 + \frac{\sf SNR}{\sf 2INR})$ & $R_{1p}$ & $\log(1 + \frac{\sf INR^2}{\sf SNR}) -2$  & $\log(\frac{1 + {\sf SNR}/{\sf INR}}{4})$   \\
 & & & & &  \\ \cline{2-6}
 & $[2/3,1]$ & $\log(1 + {\sf SNR}/{\sf 2INR})$ & $R_{1p}$  & $\log({\sf INR^2}/{\sf 3SNR})$ & $\log({\sf 2SNR}/{\sf 3INR})$  \\ \hline
 & $[0,1]$ & $\log(1 + \frac{\sf SNR}{2 {\sf INR} })$& $R_{1p}$ & 0 & $\log(\frac{{\sf INR}}{3})$  \\ \cline {2 -6}
$\mathcal{P}_{\rm D}$ & $(1,\infty)$ & 0 & 0  & 0 & $\log(1 + {\sf INR})$   \\\hline
\end{tabular}
\end{table}

The rate and power allocation to achieve within a constant number of
bits from the outer bound on the feedback model $(1000)$
are given in Tables~\ref{table:lambdas} and \ref{table:rates}. The points $\mathcal{P}_{\rm A}, \mathcal{P}_{\rm
  B}, \mathcal{P}_{\rm C}$ and $\mathcal{P}_{\rm D}$ describe four
different achievable rate pairs $(R_1,R_2)$ using the $(1000)$ feedback
model. For different $\alpha$ values, different power and rate allocations are used. The
achievable rate for the ${\sf T}_1$-${\sf D}_1$ user pair is $R_1 =
R_{1p} + R_{1c}$ and for the ${\sf T}_2$-${\sf D}_2$ user pair it is $R_2 =
R_{2p} + R_{2c}$.

\subsubsection{Achievability for $(0010)$ Feedback Model}
\label{sec:(0010)_l}
\label{sec:(0010)_l}
Here, we show the rate and power allocation for achieving a rate pair
within a constant number of bits from $\overline{\mathcal{K}}_{\rm B}$
in the $(0010)$ feedback model in the weak interference regime. At ${\sf
  T}_1$, all the power is used to transmit $X_{1i}$. The power
allocation at ${\sf T}_2$ is
\begin{eqnarray}
  \lambda_{2,d} = 1 - \frac{1}{\sf INR}, \text{ }\lambda_{2,nd} = \frac{1}{\mathsf{INR}} - \frac{\sf INR}{\sf SNR}, \text{ when } {\alpha \leq \frac{1}{2}} \label{eq:(0010)_l1}\\
  \lambda_{2,d} = 1 - \frac{1}{\sf INR}, \text{ }\lambda_{2,nd} = 0,\text{ when } {\alpha} \geq \frac{1}{2} \label{eq:(0010)_l2}
\end{eqnarray}
while the rate allocation is
\begin{eqnarray}
  R_1 &  = &  \log\left(1 + \frac{\sf SNR}{2}\right) \label{eq:(0010)_r1} \\
R_{2,d} &  =  &\log\left(\frac{\sf INR}{2}\right), \text{ }R_{2,nd}  = \log\left(\frac{\sf SNR}{{\sf2 INR}^2}\right), \text{ when } \alpha <  \frac{1}{2} \label{eq:(0010)_r21}\\
R_{2,d}  & = & \log\left(\frac{\sf SNR}{2\mathsf{INR}}\right), \text{ } R_{2,nd} = 0, \text{ when } \frac{1}{2} \leq \alpha \leq 1 \label{eq:(0010)_r22}
\end{eqnarray}

%% Here we show the rate and power allocation for achieving a rate pair
%% within constant number of bits from $\overline{\mathcal{K}}_{\rm B}$
%% in $(0010)$ feedback model in the weak interference regime. At ${\sf
%%   T}_1$, all the power is used to transmit $X_{1i}$. The power
%% allocation at ${\sf T}_2$ is
%% \begin{eqnarray}
%%   \lambda_{2,d} = \min\left(1,\frac{1}{\sf INR}\right) \label{eq:(0010)_l2}
%% \end{eqnarray}
%% while the rate allocation is
%% \begin{eqnarray}
%%   R_1  = \log\left(1 + \frac{\sf SNR}{2}\right), \text{ }R_{2} = \log\left(1 + \frac{\sf SNR}{\sf 2INR + 1 }\right) \label{eq:(0010)_r1}
%% \end{eqnarray}

 %% Note that,
%% whenever $R_{2r} = 0$, feedback is not necessary.
